# Supplementary material for: Avoiding Unbound Anions in Density Functional Calculations
Source: arXiv:1103.4467 source file (2011-03-23)
Supplement: Supplementary file 1 [file KSB11_SI.pdf]

# Avoiding Unbound Anions in Density Functional Calculations

Min-Cheol Kim,[1] Eunji Sim,[1] and Kieron Burke[2]

[1)] *Department of Chemistry and Institute of Nano-Bio Molecular Assemblies, Yonsei University, 262 Seongsanno Seodaemun-gu, Seoul 120-749 Korea*

[2)] *Department of Chemistry, University of California, Irvine, CA, 92697, USA*

(Dated: 18 March 2011)

## I. VERTICAL ELECTRON DETACHMENT DENSITY

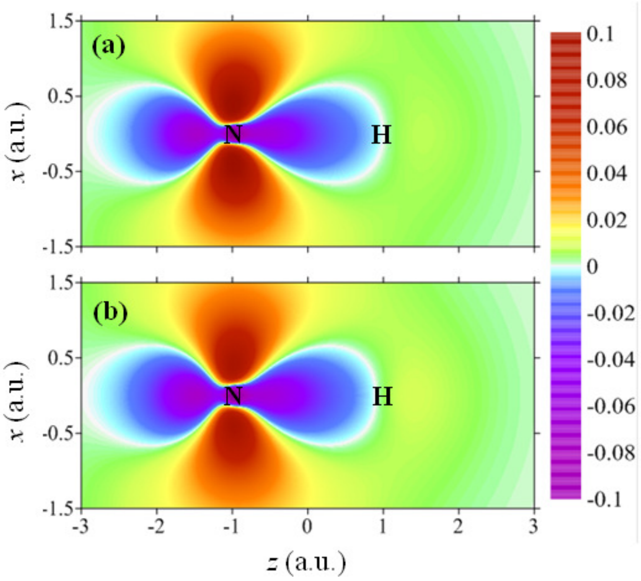


FIG. 1. Cross sections of vertical electron detachment densities (anion - neutral) along the molecular axis of (a) PBE and (b) HF plotted for NH. AVTZ basis sets are used, and the geometries are based on the anion. Atoms are placed along the $z$ axis(the molecular axis).

Vertical electron detachment density is defined as:

$$n^{\mathrm{VED}}(r) = n_{-1}^{-1}(r) - n_{-1}^{0}(r) \tag{1}$$

where $\mathrm{n}_{Q'}^{Q}$ is the charge density of species with charge $Q$, in the optimized geometry with charge $Q'$. By using the vertical electron detachment density, we eliminate the effects of geometry relaxation in the electron affinity density. In Fig 1, cross section of vertical electron detachment densities of NH is plotted along the molecular axis. There is almost no difference between Fig 3(maintext) and Fig 1, except near the N nucleus. Densities around the H atom show self-consistent densities are more diffuse than HF densities in both figures. To get more clear evidence of this, the vertical electron detachment density in Fig 1 is plotted along the principle molecule axis in fig. 2. Self-consistent density is clearly more diffuse than the HF density, illustrating the electron leakage in DFT anion calculations.

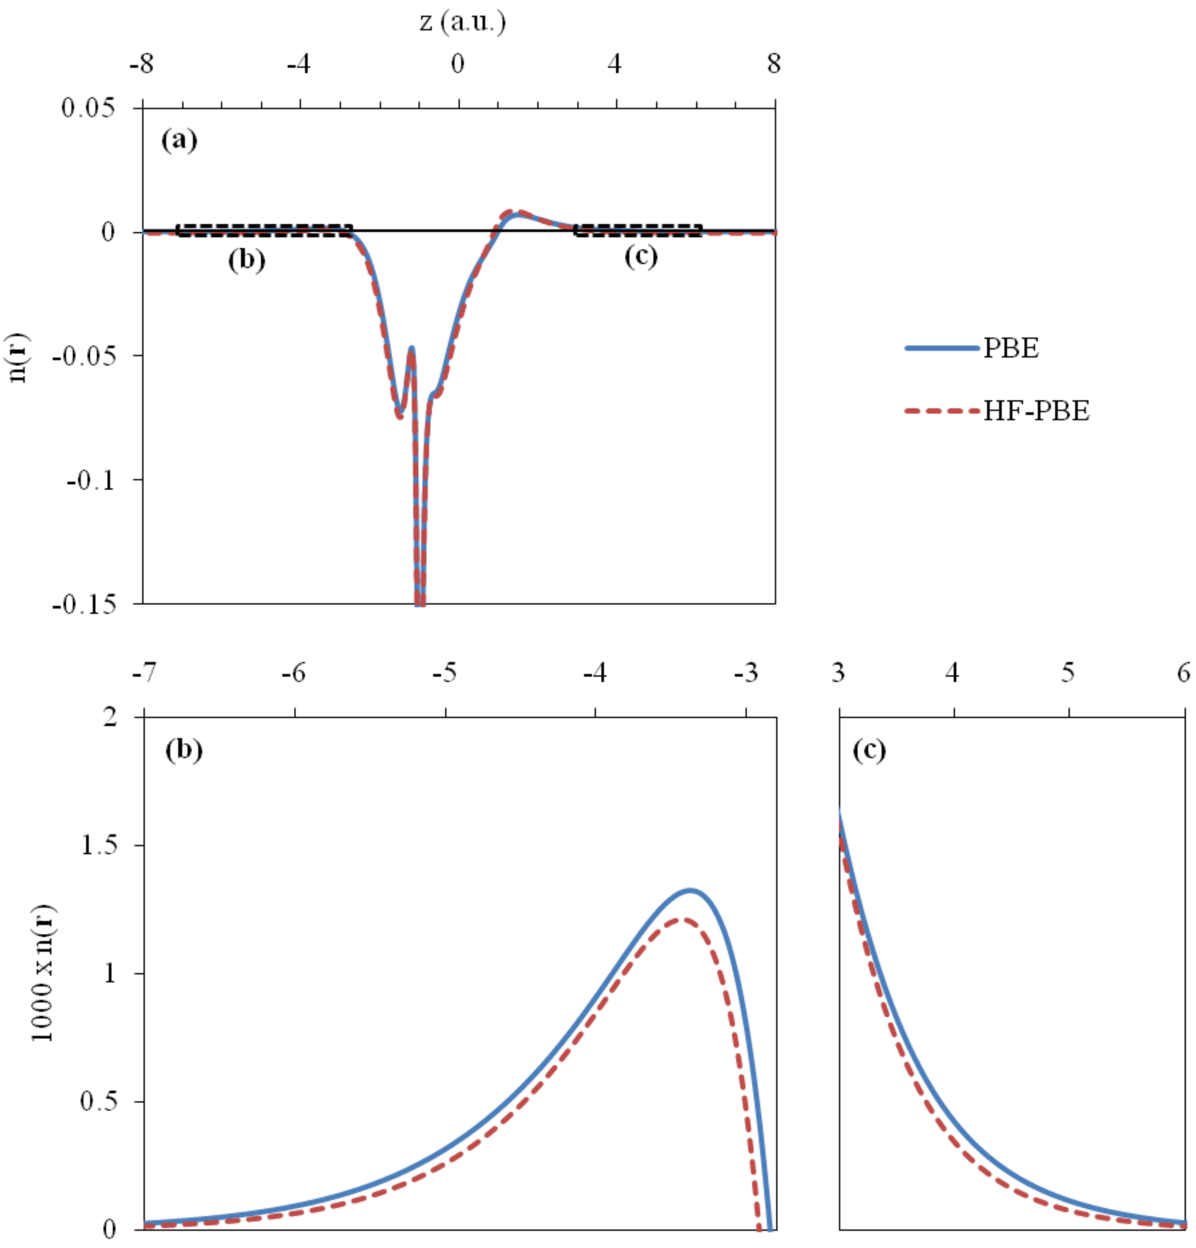


FIG. 2. Local vertical electron detachment densities (anion - neutral) along the molecular axis ($z$-axis) in Fig 1. N is positioned at $z = -0.99$ and H is at $z = 0.99$. Regions in (a) are magnified into (b) and (c) for clarity.

## II. SPIN CONTAMINATION

Spin contamination appears in unrestricted wave functions with higher spin states mixed in its desired spin state, resulting in higher energy than its ground state energy. If there is

TABLE I. Spin contamination(%) in KS-DFT and HF-DFT on G2-1 molecule set.

| Mol. | $(2s+1)$ | | Neutral | | | | Anion | | | |
|---|---|---|---|---|---|---|---|---|---|---|
| | | | MBS | | HF-DFT | | MBS | | HF-DFT | |
| | neut. | anion | PBE | B3LYP | PBE | B3LYP | PBE | B3LYP | PBE | B3LYP |
| CH | 2 | 3 | 0.4 | 0.4 | 1.3 | 1.3 | 0.3 | 0.4 | 1.2 | 1.2 |
| $CH_2$ | 3 | 2 | 0.3 | 0.3 | 0.9 | 0.8 | 0.6 | 0.8 | 2.7 | 2.8 |
| $CH_3$ | 2 | 1 | 0.5 | 0.5 | 1.6 | 1.6 | 0.0 | 0.0 | 0.0 | 0.0 |
| NH | 3 | 2 | 0.3 | 0.3 | 0.9 | 0.8 | 0.9 | 1.1 | 8.1 | 8.1 |
| $NH_2$ | 2 | 1 | 0.4 | 0.5 | 1.3 | 1.3 | 0.0 | 0.0 | 0.0 | 0.0 |
| OH | 2 | 1 | 0.3 | 0.4 | 1.0 | 1.0 | 0.0 | 0.0 | 0.0 | 0.0 |
| SiH | 2 | 3 | 0.7 | 0.7 | 3.1 | 3.1 | 0.4 | 0.3 | 1.8 | 1.8 |
| $SiH_2$ | 1 | 2 | 0.0 | 0.0 | 0.0 | 0.0 | 0.8 | 0.7 | 3.4 | 3.4 |
| $SiH_3$ | 2 | 1 | 0.4 | 0.3 | 0.7 | 0.7 | 0.0 | 0.0 | 0.0 | 0.0 |
| PH | 3 | 2 | 0.3 | 0.3 | 1.4 | 1.4 | 0.8 | 0.8 | 2.8 | 2.8 |
| $PH_2$ | 2 | 1 | 0.7 | 0.7 | 2.7 | 2.6 | 0.0 | 0.0 | 0.0 | 0.0 |
| HS | 2 | 1 | 0.6 | 0.6 | 1.9 | 1.9 | 0.0 | 0.0 | 0.0 | 0.0 |
| $O_2$ | 3 | 2 | 0.2 | 0.5 | 2.5 | 2.4 | 0.5 | 1.0 | 6.1 | 5.9 |
| NO | 2 | 3 | 0.3 | 0.5 | 9.1 | 4.9 | 0.3 | 0.6 | 2.6 | 2.6 |
| CN | 2 | 1 | 0.8 | 1.1 | 55.7 | 49.5 | 0.0 | 0.0 | 0.0 | 0.0 |
| PO | 2 | 3 | 0.5 | 0.6 | 3.2 | 3.0 | 0.2 | 0.4 | 2.3 | 2.3 |
| $S_2$ | 3 | 2 | 0.3 | 0.5 | 2.9 | 2.9 | 0.4 | 0.7 | 4.5 | 4.5 |
| $Cl_2$ | 1 | 2 | 0.0 | 0.0 | 0.0 | 0.0 | 0.3 | 0.5 | 3.1 | 3.2 |

no spin contamination, the expectation value of total spin, $\langle S^2 \rangle$, should be equal to $s(s+1)$, where $s$ is the total spin state of the system. In case of organic molecules, calculations with spin contamination more than 10% difference are not reliable[1]. If the spin contamination is too large, the density derived from the corresponding molecular orbitals is inaccurate, DFT energies evaluated on this crude density are also inaccurate.

In table I, spin contamination of our work is given as the relative error between calculated

unrestricted $\langle S^2 \rangle$ and $s(s+1)$ :

$$\text{spin contamination} = \frac{|\langle S^2 \rangle - s(s+1)|}{s(s+1)} \times 100(\%). \qquad (2)$$

## III. PBE0 ELECTRON AFFINITY ERRORS

TABLE II. PBE0 errors in electron affinity of molecules in the G2-1 molecule set excluding CN (eV).

| EA | Mol. | PBE0 | HF-PBE0 | EA | Mol. | PBE0 | HF-PBE0 |
|---|---|---|---|---|---|---|---|
| 1.24 | CH | 0.15 | 0.12 | 1.03 | PH | -0.06 | -0.06 |
| 0.65 | $CH_2$ | -0.10 | -0.13 | 1.27 | $PH_2$ | -0.10 | -0.09 |
| 0.08 | $CH_3$ | -0.14 | -0.16 | 2.36 | HS | -0.12 | -0.11 |
| 0.38 | NH | -0.14 | -0.20 | 0.44 | $O_2$ | -0.16 | -0.19 |
| 0.77 | $NH_2$ | -0.22 | -0.24 | 0.02 | NO | 0.20 | 0.11 |
| 1.83 | OH | -0.23 | -0.28 | 3.86 | CN | 0.04 | 0.64 |
| 1.28 | SiH | 0.09 | 0.08 | 1.09 | PO | 0.20 | 0.19 |
| 1.12 | $SiH_2$ | 0.14 | 0.12 | 1.66 | $S_2$ | -0.05 | -0.03 |
| 1.41 | $SiH_3$ | -0.09 | -0.08 | 2.39 | $Cl_2$ | 0.22 | 0.22 |

| MAE | | ME | |
|---|---|---|---|
| PBE0 | HF-PBE0 | PBE0 | HF-PBE0 |
| 0.14 | 0.14 | -0.02 | -0.04 |

PBE0 is a parameter-free hybrid functional[2] using exact exchange of 25% in the PBE functional[3]. To further check the performance of HF-DFT in hybrid functionals, we compared the electron density errors between MBS and HF-DFT using PBE0 in Table II. As expected, the MAE of HF-PBE0 is similar with PBE0, while the ME is more negative.

## REFERENCES


[1]D. Young, *Computational Chemistry: A Practical Guide for Applying Techniques to Real World Problems* (John Wiley & Sons, Inc., 2001).

[2]J. P. Perdew, M. Ernzerhof, and K. Burke, "Rationale for mixing exact exchange with density functional approximations," J. Chem. Phys., **105**, 9982 (1996).

[3]J. P. Perdew, K. Burke, and M. Ernzerhof, “Generalized gradient approximation made simple,” Phys. Rev. Lett., **77**, 3865 (1996)

[1]D. Young, *Computational Chemistry: A Practical Guide for Applying Techniques to Real World Problems* (John Wiley & Sons, Inc., 2001).

[2]J. P. Perdew, M. Ernzerhof, and K. Burke, “Rationale for mixing exact exchange with density functional approximations,” J. Chem. Phys., **105**, 9982 (1996).

[3]J. P. Perdew, K. Burke, and M. Ernzerhof, “Generalized gradient approximation made simple,” Phys. Rev. Lett., **77**, 3865 (1996).
